# Supplementary material for: GSNs : Generative Stochastic Networks
Source: arXiv:1503.05571 source file (2015-03-23)
Supplement: Supplementary file 1 [file supplemental.tex]

%%%%%%%%%%%%%%%%%%%%%%%%%%%%%%%%%%%%%%%%%%%%%%%%%%%%%%%%%%%%%%%%%%
%%%%%%%% ICML 2014 EXAMPLE LATEX SUBMISSION FILE %%%%%%%%%%%%%%%%%
%%%%%%%%%%%%%%%%%%%%%%%%%%%%%%%%%%%%%%%%%%%%%%%%%%%%%%%%%%%%%%%%%%

% Use the following line _only_ if you're still using LaTeX 2.09.
%\documentstyle[icml2014,epsf,natbib]{article}
% If you rely on Latex2e packages, like most moden people use this:
\documentclass{article}

% use Times
\usepackage{times}
% For figures
\usepackage{graphicx} % more modern
\usepackage{subfigure} 

% For citations
\usepackage{natbib}

% For algorithms
\usepackage{algorithm}
\usepackage{algorithmic}

% As of 2011, we use the hyperref package to produce hyperlinks in the
% resulting PDF.  If this breaks your system, please commend out the
% following usepackage line and replace \usepackage{icml2014} with
% \usepackage[nohyperref]{icml2014} above.
\usepackage{hyperref}

% Packages hyperref and algorithmic misbehave sometimes.  We can fix
% this with the following command.

% Employ the following version of the ``usepackage'' statement for
% submitting the draft version of the paper for review.  This will set
% the note in the first column to ``Under review.  Do not distribute.''
%\usepackage{icml2014}
% Employ this version of the ``usepackage'' statement after the paper has
% been accepted, when creating the final version.  This will set the
% note in the first column to ``Proceedings of the...''
\usepackage[accepted]{icml2014}

% JBY
% Custom packages / etc.
\usepackage[utf8]{inputenc}
\usepackage{booktabs}
\usepackage{amsthm}
\usepackage{amsmath}  % required if you use \overset
\usepackage{xr} % to refer to external references from the main paper
\externaldocument{main}
\usepackage{ownstyles}

\newif\ifLongversion
\Longversionfalse

% We input some notation formatting to allow shared formatting between the main paper and the supplemental section
\input{notation}

% The \icmltitle you define below is probably too long as a header.
% Therefore, a short form for the running title is supplied here:
\icmltitlerunning{Supplemental Material for: Deep Generative Stochastic Networks Trainable by Backprop}

\begin{document} 

\twocolumn[
\icmltitle{Supplemental Material for: Deep Generative Stochastic Networks Trainable by Backprop}

% It is OKAY to include author information, even for blind
% submissions: the style file will automatically remove it for you
% unless you've provided the [accepted] option to the icml2014
% package.

% We input the author info so we can store the authors for the main and supplemental parts in the same location
\input{authors}

% You may provide any keywords that you 
% find helpful for describing your paper; these are used to populate 
% the "keywords" metadata in the PDF but will not be shown in the document
\icmlkeywords{deep learning, unsupervised learning, generative models, denoising autoencoder}

\vskip 0.3in
]

\input{supplemental_body}

%\bibliography{strings,strings-shorter,ml,aigaion-shorter,cultrefs}
%\bibliographystyle{icml2014}

{\small
\bibliography{strings,strings-shorter,ml,aigaion-shorter,cultrefs}
\bibliographystyle{icml2014}
}

\end{document}
